# Supplementary material for: Strong thermal fluctuations in cuprate superconductors in magnetic field above Tc
Source: arXiv:1307.7358 source file (2013-07-28)
Supplement: Supplementary file 1 [file Supplmat.pdf]

# Supplementary Material for "Strong thermal fluctuations in cuprate superconductors in magnetic field above $T_c$"

Xujiang Jiang[1], Dingping Li[1], Baruch Rosenstein[2]
[1]School of Physics, Peking University, Beijing 100871, China. and
[2]Electrophysics Department, National Chiao Tung University, Hsinchu 30050, Taiwan, R. O. C.
(Dated: July 28, 2013)

In this supplementary information, we provide more details about self consistent approximation theory and its application to the magnetization in type $II$ superconductors.

## I. THE SELF CONSISTENT APPROXIMATION.

The self consistent approximation theory (SCFT, also sometimes called variational Gaussian approximation theory) can be presented in many different ways. Here we use a variational (minimal sensitivity principle[1]) derivation along the lines of the more general "optimized expansion"[2]. Here we apply it to calculate the fluctuation magnetization of the type II superconductor described within the GL approach by free energy, Eq.(1). The partition function is the functional integral over the Boltzmann factor Eq.(2)

$$Z=\int \mathcal{D}\psi\mathcal{D}\psi^{*}\exp\left(-f[\psi]\right) \tag{S1}$$

Within The Boltzmann factor $f[\psi]$ is divided into an optimized quadratic ("large") part $K[\psi,\varepsilon]$ and a small perturbation $W[\psi,\varepsilon]$, where $\varepsilon$ is the variational parameter, the vortex liquid gap in our case. Then the free energy is expanded to first order in $W$:

$$\begin{aligned} F\left(\varepsilon\right) &= -T\ln Z=-T\ln\int_{\psi}\exp\left[-\left(K+W\right)\right] \\ &= -T\ln\int_{\psi}e^{-K}\left(1-W\right)=-T\ln Z_{0}+T\langle W\rangle_{0}. \end{aligned} \tag{S2}$$

Here unperturbed quantities $Z_0$ and $\langle W\rangle_0$ are defined as

$$Z_{0}=\int_{\psi}e^{-K},\qquad \langle W\rangle_{0}=Z_{0}^{-1}\int_{\psi}We^{-K}. \tag{S3}$$

The gap equation, determining $\varepsilon$ variationally, is

$$\frac{d}{d\varepsilon}F\left(\varepsilon\right)=0. \tag{S4}$$

The method is very general, but the psesence of magnetic field and UV cutoff makes its application nontrivial.

## II. MAGNETIZATION OF THE LAWRENCE-DONIACH GL MODEL IN STRONGLY TYPE II SUPERCONDUCTORS

Gibbs energy of Lawrence Doniach model is

$$G\left[\psi,A\right]=s^{\prime}\sum_{l}\int_{\mathbf{r}}\left[\frac{\hbar^{2}}{2m_{a}}\left|\mathbf{D}\psi_{l}\right|^{2}+\frac{\hbar^{2}}{2m_{c}d^{\prime2}}\left|\psi_{l}-\psi_{l+1}\right|^{2}+\alpha\left(T-T_{\Lambda}\right)\left|\psi_{l}\right|^{2}+\frac{\beta}{2}\left|\psi_{l}\right|^{4}+\frac{\left(B_{l}-H\right)^{2}}{8\pi}\right]. \tag{S5}$$

For constant homogeneous external magnetic field, we shall calculate partition function of the Gibbs ensemble,

$$Z=\int\mathcal{D}\mathbf{A}\mathcal{D}\psi\mathcal{D}\psi^{*}e^{-G[\psi,A]/T}. \tag{S6}$$

Performing the same rescaling of fields as in the Letter, the Boltzmann weight becomes: $g\equiv G/T=f\left[\phi,b\right]+f_{mag}\left[b\right]$, where $f$ is given in Eq.(2) and

$$f_{mag}\left[b\right]=\frac{\kappa^{2}}{4\omega_{\Lambda}t_{\Lambda}}\sum_{l}\int_{\mathbf{r}}\left(b_{l}-h\right)^{2}. \tag{S7}$$

Therefore thermodynamic (effective) Gibbs energy density,

$$\mathcal{G}=-d\omega_{\Lambda}t_{\Lambda}V^{-1}\ln Z, \tag{S8}$$

defined as dimensionless thermodynamic Gibbs energy which determines the magnetization inside superconducting layer $\left\langle b_{l}-h\right\rangle/\left(4\pi\right)$ via

$$\left\langle b_{l}-h\right\rangle/\left(4\pi\right)=-\frac{1}{2\pi\kappa^{2}}\frac{\partial\left(\mathcal{G}\left(h\right)\right)}{\partial h}=-\frac{d}{4\pi V}Z^{-1}\int_{\mathbf{A},\psi}\sum_{l}\int_{\mathbf{r}}\left(b_{l}-h\right)e^{-G[\psi,A]/T}. \tag{S9}$$

Since $\kappa>>1$ magnetization is small $\left\langle b_{l}-h\right\rangle/\left(4\pi\right)\sim\kappa^{-2}h$, and it suffice to consider a simpler statistical sum

$$Z\approx\int_{\phi}e^{-f[\phi,h]}. \tag{S10}$$

Thermodynamic Gibbs energy density $\mathcal{G}\left(h\right)$ in $\frac{\partial(\mathcal{G}(h))}{\partial h}$of Eq.(S9) can be approximated as $-d\omega_{\Lambda}t_{\Lambda}V^{-1}\ln Z$ where $Z$ is given in Eq.(S10). Next we will use the self consistent approximation to calculate $\ln Z$.

## III. APPLICATION OF THE SELF-CONSISTENT METHOD IN THE PRESENCE OF MAGNETIC FIELD

We take $f\left[\phi,b\right]=K+W$ as defined in the letter Eqs.(3, 4). The zero order partition function $Z_0$ is the form of gaussian functional integral. The order parameter $\phi_l(r)$ is expanded in eigenfunctions [3],

$$\phi_{l}(r)=\frac{1}{\left(2\pi\right)^{3/2}}\sum_{n}\int_{\mathbf{q}}\int_{k=0}^{2\pi/d}e^{ildk}\varphi_{n,\mathbf{q}}\phi_{k,\mathbf{q},n}, \tag{S11}$$

where $k$ is the wave vector in $c$ direction and $\varphi_{n,\mathbf{q}}$ is the Landau's quasi - momentum wave function that obeys

$$-\frac{1}{2}\mathbf{D}^{2}\varphi_{n,\mathbf{q}}=\left(n+\frac{1}{2}\right)b\varphi_{n,\mathbf{q}}. \tag{S12}$$

The $\mathbf{q}$ integration is over the Abrikosov lattice Brillouin zone (applicable even when the lattice melts [3]) with area $2\pi b$. In this basis

$$Z_{0}=\int_{\psi}\exp\left\{-\frac{1}{\omega_{\Lambda}t_{\Lambda}d}\sum_{n=0}^{\infty}\int_{\mathbf{q}}\int_{k=0}^{2\pi/d}\left[\frac{1}{d^{2}}(1-\cos(kd))+nb+\varepsilon\right]\phi_{k,\mathbf{q},n}\phi_{k,\mathbf{q},n}^{*}\right\} \tag{S13}$$

The gaussian integral results in

$$\ln Z_{0}=-\frac{Vb}{(2\pi)^{2}}\int_{k=0}^{2\pi/d}\sum_{n=0}^{N_{\max}(\Lambda)}\ln\left[\frac{1}{d^{2}}(1-\cos(kd))+nb+\varepsilon\right]. \tag{S14}$$

It is not apriori clear how to "trade" the energy cutoff $\Lambda$ to maximal Landau level. However the physical requirement of "renormalizability" of the SCFT, namely that a physical quantity should be cutoff independent near criticality. This unambiguously leads to

$$(N_{f}+1)b=\Lambda. \tag{S15}$$

With this upper limit the sum can be done

$$\mathcal{G}_{0}/V=-V^{-1}d\omega_{\Lambda}t_{\Lambda}\ln Z=\frac{d\omega_{\Lambda}t_{\Lambda}b}{(2\pi)^{2}}\int_{k=0}^{2\pi/d}\left[\frac{\Lambda}{b}\ln b+\ln\Gamma\left(g+\Lambda/b\right)-\ln\Gamma\left(g\right)\right], \tag{S16}$$

where $g$ is given in Eq.(5).

It is convenient to express the average of the superfluid density via derivative with respect to variational parameter:

$$\left\langle |\phi_l|^2 \right\rangle_0 = Z_0^{-1} \int_\phi |\phi_l|^2 e^{-K} = \frac{\partial}{\partial \varepsilon} \left( \mathcal{G}_0 / V \right) = \frac{d\omega_\Lambda t_\Lambda}{(2\pi)^2} \int_{k=0}^{2\pi/d} \left[ \psi \left( g + \Lambda / b \right) - \psi \left( g \right) \right]. \tag{S17}$$

Combining the Eq. (S2), Eq. (S16) and Eq. (S17) we finally arrive at the free energy of the system,

$$\mathcal{G}/V = \mathcal{G}_0/V - \left( \varepsilon + \frac{1 - t_\Lambda - b}{2} \right) \frac{\partial \left( \mathcal{G}_0/V \right)}{\partial \varepsilon} + \left( \frac{\partial \mathcal{G}_0/V}{\partial \varepsilon} \right)^2. \tag{S18}$$

The gap equation, Eq.(5) of the main text is obtained by optimizing the free energy, $\partial \mathcal{G}/\partial \varepsilon = 0$.

Taking $b = 0$ in Eq.(5), the gap equation without magnetic field Eq.(6) is obtained. The renormalized transition temperature $T_c$ is arrived at $b = 0$, by requiring criticality, $\varepsilon = 0$ in Eq.(6), see Eq.(7). The gap equation can be expressed through the renormalized transition temperature $T_c$, Eq.(8) by using Eq.(7).

The magnetization is $\left\langle b_l - h \right\rangle / (4\pi)$ inside the superconducting layer, therefore the average magnetization in the whole sample is $(s/d) \left\langle b_l - h \right\rangle / (4\pi)$. $\left\langle b_l - h \right\rangle / (4\pi)$ can be obtained by Eq.(S9) and Eq.(S18). The results can be found in the main text Eq.(10).


[1] P. M. Stevenson, Phys. Rev. D **30**, 1712 (1984); A. Kovner and B. Rosenstein, Phys. Rev. D **39**, 2332 (1989).

[2] D. Li and B. Rosenstein, Phys. Rev. B **65**, 024513 (2001); H. Kleinert, Path Integrals in Quantum Mechanics, Statistics, Polymer Physics, and Financial Markets, (World Scientific, Singapore, 2009).

[3] B. Rosenstein and D. Li, Rev. Mod. Phys. **82**, 109 (2010).
